# Supplementary material for: The Ornstein-Uhlenbeck process with migration: evolution with interactions
Source: arXiv:1607.07970 source file (2016-07-27)

# Supplementary material

## The Ornstein–Uhlenbeck process with migration: evolution with interactions

Krzysztof Bartoszek      Sylvain Glémin      Ingemar Kaj      Martin Lascoux

| Setup id | $\alpha$ | $m$ | $\theta_1$ | $\theta_2$ | Setup id | $\alpha$ | $m$ | $\theta_1$ | $\theta_2$ |
|----------|----------|-----|------------|------------|----------|----------|-----|------------|------------|
| 1        | 0.5      | 0   | 0          | 0          | 2        | 1        | 0   | 0          | 0          |
| 3        | 10       | 0   | 0          | 0          | 4        | 0.5      | 0.1 | 0          | 0          |
| 5        | 1        | 0.1 | 0          | 0          | 6        | 10       | 0.1 | 0          | 0          |
| 7        | 0.5      | 0.5 | 0          | 0          | 8        | 1        | 0.5 | 0          | 0          |
| 9        | 10       | 0.5 | 0          | 0          | 10       | 0.5      | 1   | 0          | 0          |
| 11       | 1        | 1   | 0          | 0          | 12       | 10       | 1   | 0          | 0          |
| 13       | 0.5      | 10  | 0          | 0          | 14       | 1        | 10  | 0          | 0          |
| 15       | 10       | 10  | 0          | 0          | 16       | 0.5      | 0   | 5          | 5          |
| 17       | 1        | 0   | 5          | 5          | 18       | 10       | 0   | 5          | 5          |
| 19       | 0.5      | 0.1 | 5          | 5          | 20       | 1        | 0.1 | 5          | 5          |
| 21       | 10       | 0.1 | 5          | 5          | 22       | 0.5      | 0.5 | 5          | 5          |
| 23       | 1        | 0.5 | 5          | 5          | 24       | 10       | 0.5 | 5          | 5          |
| 25       | 0.5      | 1   | 5          | 5          | 26       | 1        | 1   | 5          | 5          |
| 27       | 10       | 1   | 5          | 5          | 28       | 0.5      | 10  | 5          | 5          |
| 29       | 1        | 10  | 5          | 5          | 30       | 10       | 10  | 5          | 5          |
| 31       | 0.5      | 0   | 0          | 5          | 32       | 1        | 0   | 0          | 5          |
| 33       | 10       | 0   | 0          | 5          | 34       | 0.5      | 0.1 | 0          | 5          |
| 35       | 1        | 0.1 | 0          | 5          | 36       | 10       | 0.1 | 0          | 5          |
| 37       | 0.5      | 0.5 | 0          | 5          | 38       | 1        | 0.5 | 0          | 5          |
| 39       | 10       | 0.5 | 0          | 5          | 40       | 0.5      | 1   | 0          | 5          |
| 41       | 1        | 1   | 0          | 5          | 42       | 10       | 1   | 0          | 5          |
| 43       | 0.5      | 10  | 0          | 5          | 44       | 1        | 10  | 0          | 5          |
| 45       | 10       | 10  | 0          | 5          | 46       | 0.5      | 0   | −5         | 5          |
| 47       | 1        | 0   | −5         | 5          | 48       | 10       | 0   | −5         | 5          |
| 49       | 0.5      | 0.1 | −5         | 5          | 50       | 1        | 0.1 | −5         | 5          |
| 51       | 10       | 0.1 | −5         | 5          | 52       | 0.5      | 0.5 | −5         | 5          |
| 53       | 1        | 0.5 | −5         | 5          | 54       | 10       | 0.5 | −5         | 5          |
| 55       | 0.5      | 1   | −5         | 5          | 56       | 1        | 1   | −5         | 5          |
| 57       | 10       | 1   | −5         | 5          | 58       | 0.5      | 10  | −5         | 5          |
| 59       | 1        | 10  | −5         | 5          | 60       | 10       | 10  | −5         | 5          |

Table S.1: Simulation setups, population size  $n = 300$ .  $\theta_1$  is the optimum for individuals  $1, \dots, 150$  and  $\theta_2$  is the optimum for individuals  $151, \dots, 300$ . In all simulations  $X_0 = 0$  and  $\sigma^2 = 1$ . In the following histograms we present the trait values inside the simulated population for all the setups.

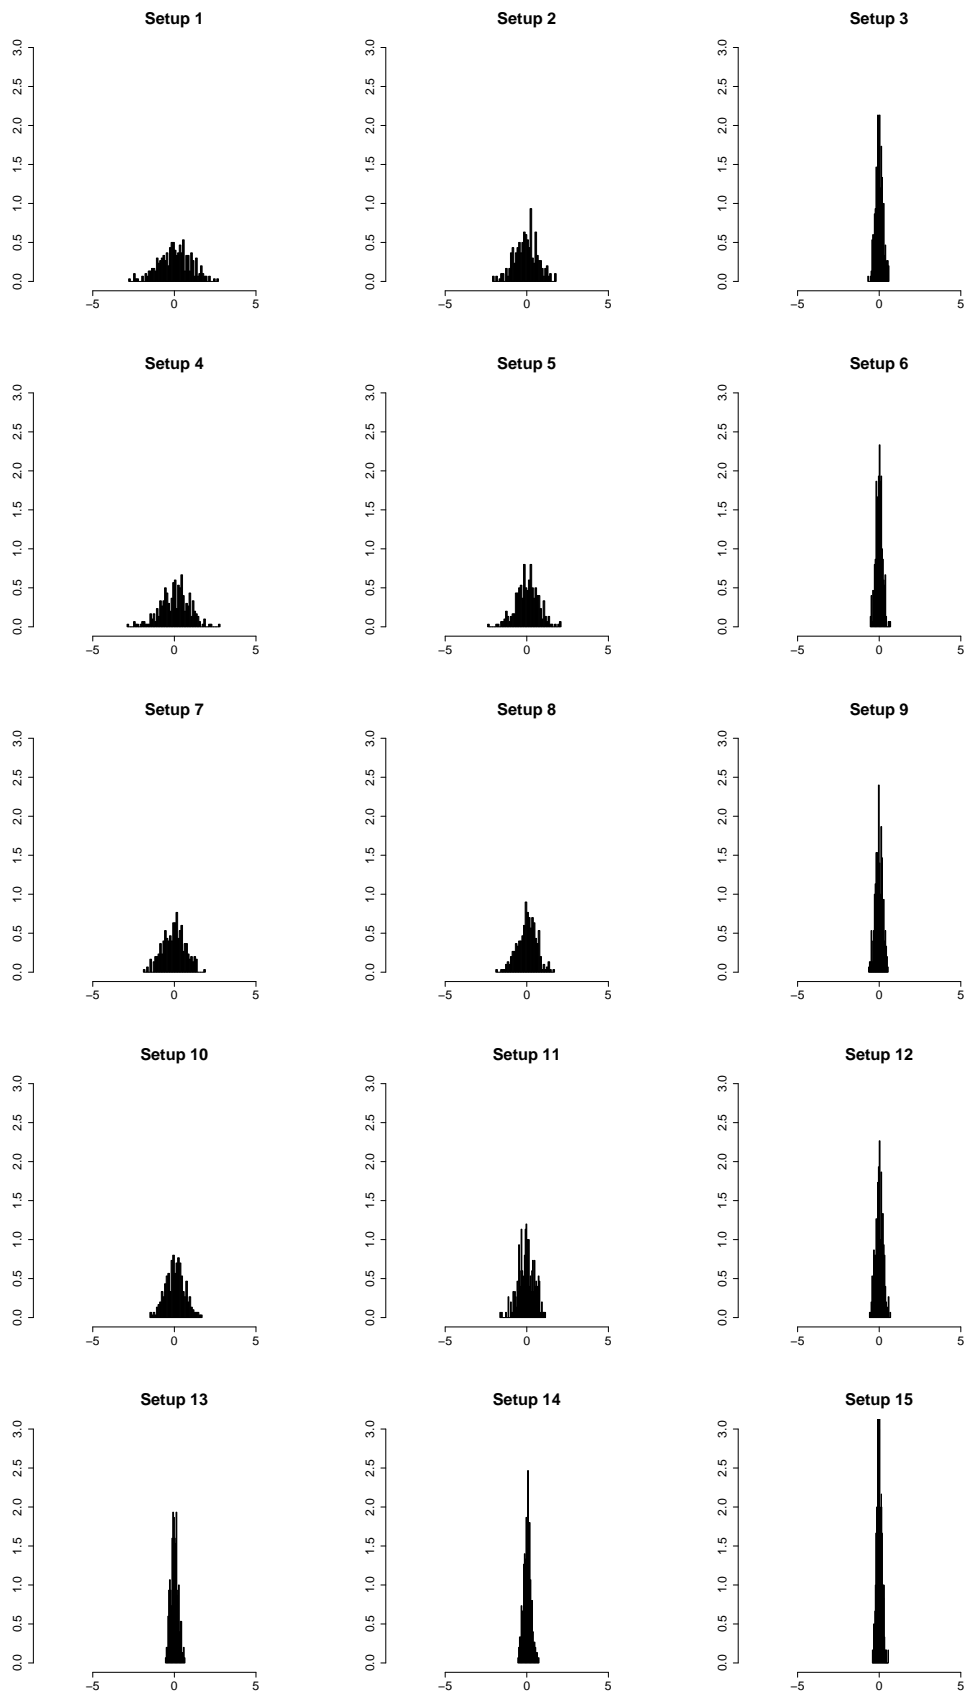

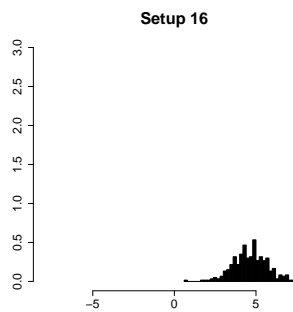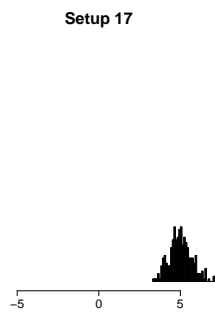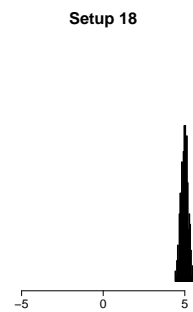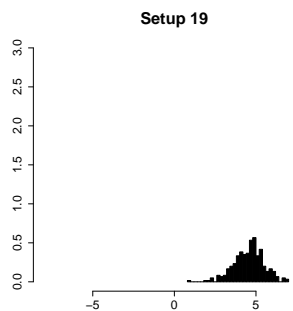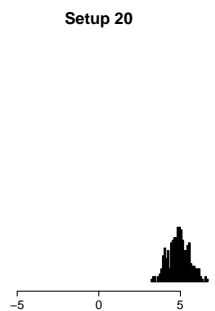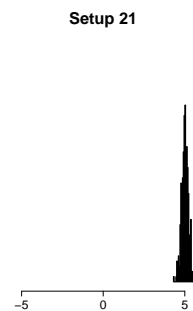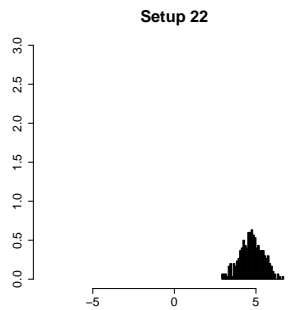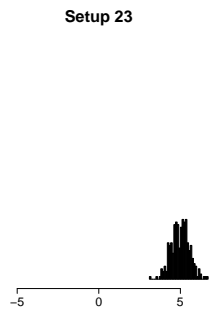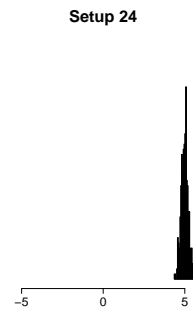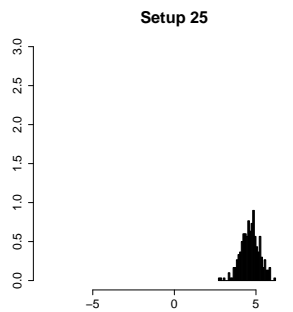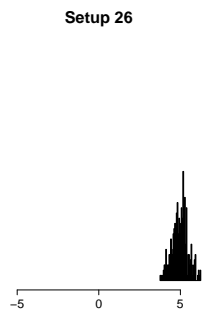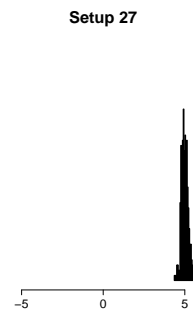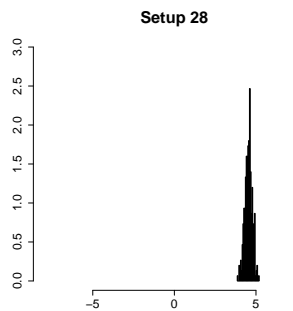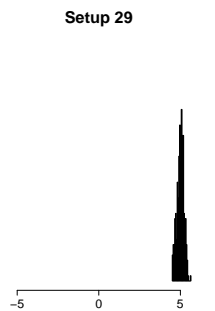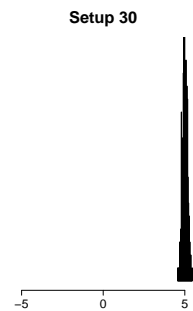

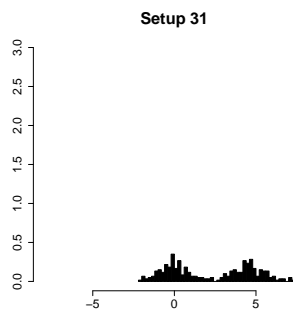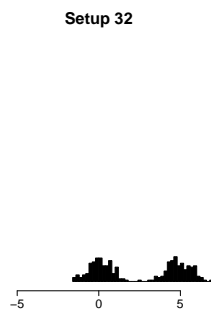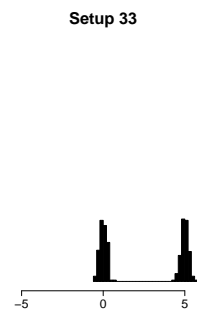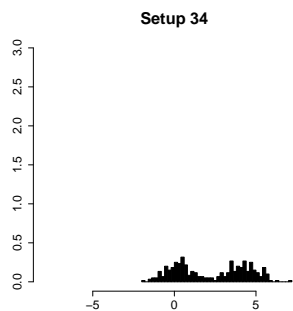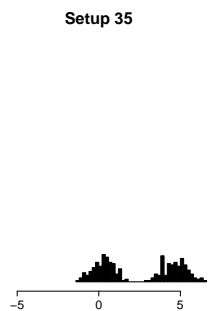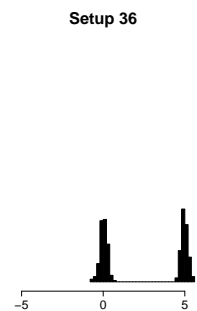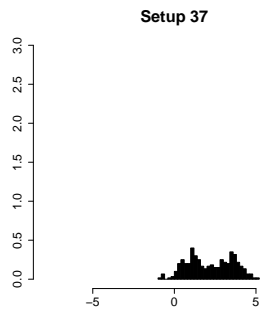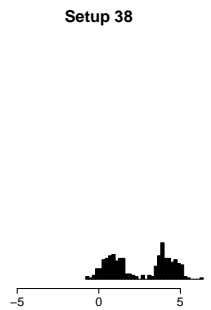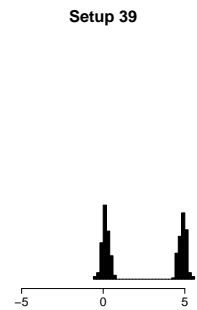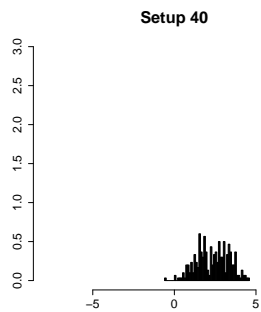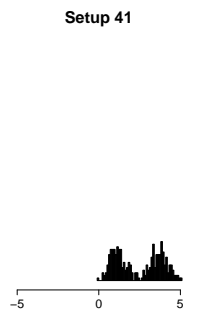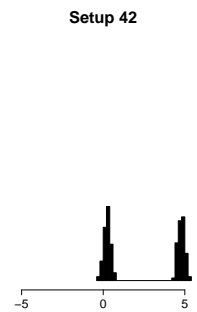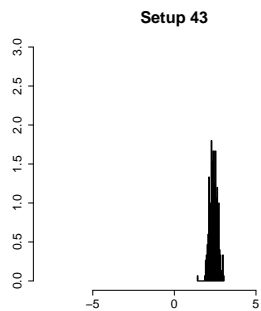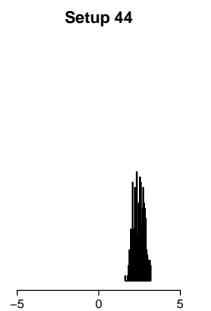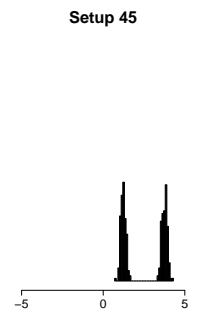

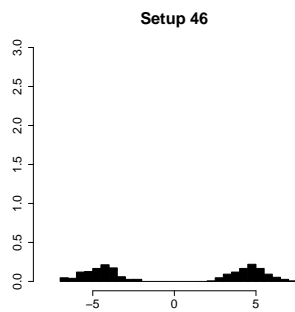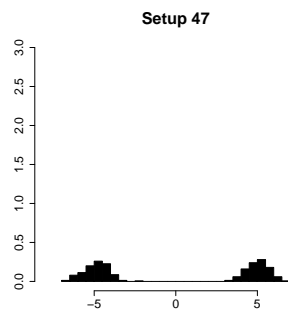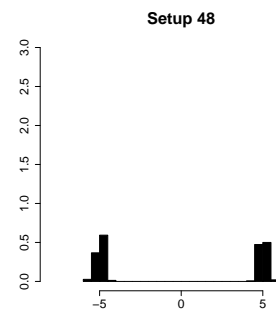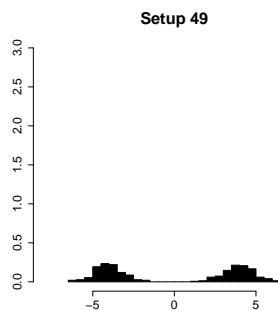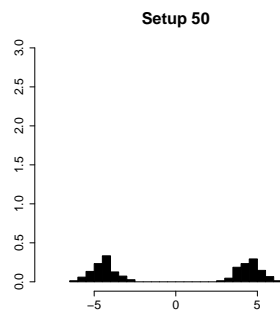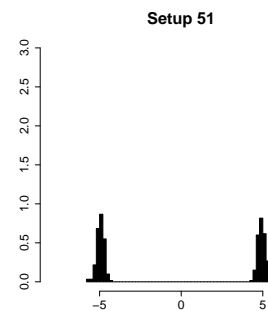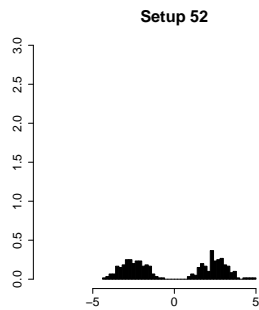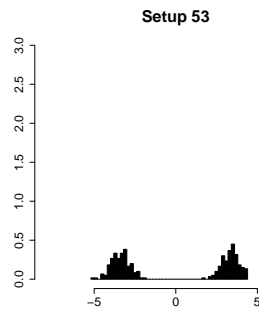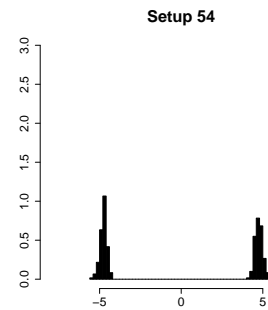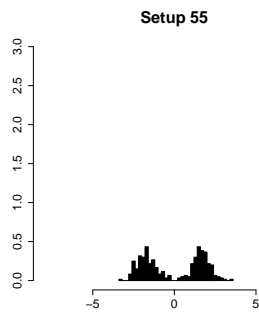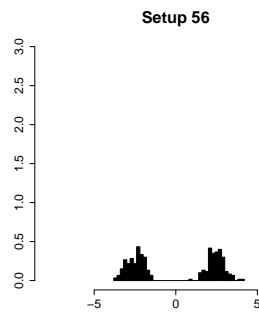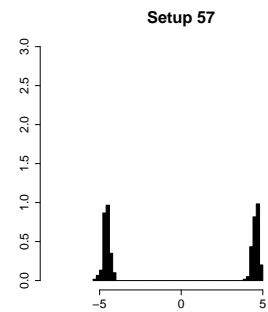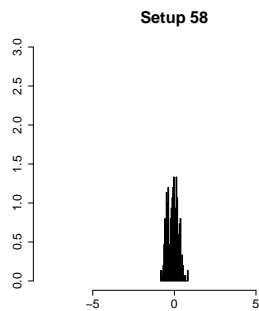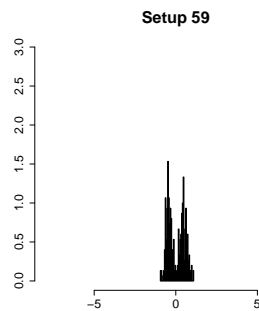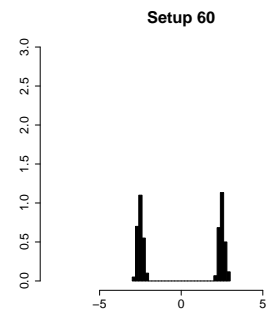

Supplement: Supplementary file 1 [file MigrationOU_Supplement.pdf]
